# Supplementary material for: $Q_B$-Optimal Two-Level Designs
Source: arXiv:2504.05072 source file (2025-04-07)
Supplement: Supplementary file 1 [file QB2level25_supplmentary.tex]

\documentclass[11pt]{article}
\usepackage[T1]{fontenc}
\usepackage{amsfonts}
\usepackage{amsmath,amsthm, amssymb}%, mathtools}
\usepackage{authblk, enumerate,natbib}
\usepackage{multicol}
\usepackage{graphicx} 
\usepackage{fancyvrb}
\usepackage{geometry}
 \geometry{
 a4paper,
 total={160mm,250mm},
 top=15mm,
 }

%%##QBmaincoord.R
%%##QB2mdcoord.R
%%##HadtoBK4.R

% Define a new Verbatim environment with modified spaceskip

%\begin{verbnobox}[\fontsize{8pt}{8pt}\selectfont]

\def\be{\begin{enumerate}} % Begin Enumerate
\def\ee{\end{enumerate}} % End Enumerate
\def\en{\item} % ENtry (item)

\setlength{\columnsep}{-2cm}
\setlength\parindent{0pt}
\setlength{\parskip}{0pt}

\title{Supplementary material for $Q_B$-optimal two-level designs}
\author[1]{Pi-Wen Tsai}
\affil[1]{National Taiwan Normal University}
\author[2]{Steven G.\ Gilmour}
\affil[2]{King's College London}
\date{}
\date{\vspace{-2.5em}}

\begin{document}
\maketitle
%$\section*{New class of $Q_B$ designs constructed by exchange algorithm}

This supplementary file gives details of the $Q_B$ designs constructed by the exchange algorithm for different cases discussed in the paper.
\be[{Case} 1:] 
\en  Supersaturated designs with $m=14$ and $N=12$
\en  Saturated main-effects designs with $m=9$ and $N=10$.
\en Unsaturated main-effects designs  with  $m = 12$ and $N = 14$.
%\en Designs for second-order maximal model with $m=4$ and $N=12$.
\en Three second-order $Q_B$-optimal designs with $m=6$ and $N=16$.
\en Two second-order $Q_B$-optimal designs  designs with $m=7$ and $N=24$.
\ee
\pagebreak

\subsection*{Case 1:  $m=14$ and $N=12$}
Designs and the corresponding matrices $X^\top X$ of the three designs in Table 1 and another two designs generated by the coordinate exchange algorithm.

  \be\itemsep=0pt
  \en $d_1$: $(b_1, b_2)=(0, 8/3)$ with 14 level-balanced factors
  
\begin{scriptsize}
\begin{multicols}{2}
\begin{verbatim}


  A  B  C  D  E  F  G  H  I  J  K  L  M  N
  1  1  1  1  1 -1  1 -1 -1  1  1 -1  1 -1
  1  1  1 -1 -1 -1  1  1  1 -1  1 -1 -1  1
 -1  1 -1 -1  1  1  1 -1  1 -1 -1 -1  1  1
  1 -1  1  1  1 -1 -1 -1 -1 -1 -1  1 -1  1
  1 -1 -1 -1 -1 -1  1  1 -1 -1 -1  1  1 -1
 -1 -1  1  1 -1  1  1  1 -1  1 -1 -1  1  1
 -1  1 -1  1  1  1 -1  1 -1 -1  1 -1 -1 -1
 -1 -1 -1  1  1 -1 -1  1  1  1  1  1  1  1
 -1  1 -1  1 -1 -1  1 -1  1  1 -1  1 -1 -1
 -1 -1  1 -1 -1  1 -1 -1  1 -1  1  1  1 -1
  1 -1  1 -1  1  1 -1  1  1  1 -1 -1 -1 -1
  1  1 -1 -1 -1  1 -1 -1 -1  1  1  1 -1  1



      A  B  C  D  E  F  G  H  I  J  K  L  M  N
  12  0  0  0  0  0  0  0  0  0  0  0  0  0  0
A  0 12  0  4 -4  0 -4  0  0 -4  0  0  0 -4  0
B  0  0 12 -4  0  0  0  4 -4  0  0  4 -4 -4  0
C  0  4 -4 12  0  0  0  0  0  0  0  0 -4  0  0
D  0 -4  0  0 12  4 -4  0  0 -4  4  0  0  0  0
E  0  0  0  0  4 12  0 -4  0  0  0  0 -4  0  0
F  0 -4  0  0 -4  0 12 -4  0  0  0  0 -4  0  0
G  0  0  4  0  0 -4 -4 12  0  0  0 -4 -4  4  0
H  0  0 -4  0  0  0  0  0 12  0  0  0 -4  0  0
I  0 -4  0  0 -4  0  0  0  0 12  0  0  0  0  0
J  0  0  0  0  4  0  0  0  0  0 12  0  0  0  0
K  0  0  4  0  0  0  0 -4  0  0  0 12  0  0  0
L  0  0 -4 -4  0 -4 -4 -4 -4  0  0  0 12  0  0
M  0 -4 -4  0  0  0  0  4  0  0  0  0  0 12  0
N  0  0  0  0  0  0  0  0  0  0  0  0  0  0 12
\end{verbatim}
\end{multicols}
\end{scriptsize}

\en $d_2$: $(b_1, b_2)=(2/9,19/9)$ with 6 level-balanced factors.

\begin{scriptsize}
\begin{multicols}{2}
\begin{verbatim}

  A  B  C  D  E  F  G  H  I  J  K  L  M  N
  1  1  1  1  1  1  1  1  1  1  1  1  1  1
  1  1  1  1 -1 -1 -1 -1  1  1 -1 -1 -1 -1
  1  1 -1 -1  1  1 -1 -1 -1 -1  1  1 -1 -1
  1  1 -1 -1 -1 -1  1  1 -1 -1 -1 -1  1  1
 -1 -1  1  1  1  1 -1 -1 -1 -1 -1 -1  1  1
 -1 -1  1  1 -1 -1  1  1 -1 -1  1  1 -1 -1
 -1 -1 -1 -1  1  1  1  1  1  1 -1 -1 -1 -1
 -1 -1 -1 -1 -1 -1 -1 -1  1  1  1  1  1  1
  1 -1  1 -1  1 -1  1 -1  1 -1  1 -1  1 -1
  1 -1  1 -1 -1  1 -1  1  1 -1 -1  1 -1  1
  1 -1 -1  1  1 -1 -1  1 -1  1  1 -1 -1  1
 -1  1  1 -1  1 -1 -1  1 -1  1 -1  1  1 -1




      A  B  C  D  E  F  G  H  I  J  K  L  M  N
  12  2 -2  2 -2  2 -2 -2  2  0  0  0  0  0  0
A  2 12  4  0  0  0  0  0  0  2 -2  2 -2 -2  2
B -2  4 12  0  0  0  0  0  0 -2  2 -2  2  2 -2
C  2  0  0 12  4  0  0  0  0  2 -2 -2  2  2 -2
D -2  0  0  4 12  0  0  0  0 -2  2  2 -2 -2  2
E  2  0  0  0  0 12  4  0  0 -2  2  2 -2  2 -2
F -2  0  0  0  0  4 12  0  0  2 -2 -2  2 -2  2
G -2  0  0  0  0  0  0 12  4  2 -2  2 -2  2 -2
H  2  0  0  0  0  0  0  4 12 -2  2 -2  2 -2  2
I  0  2 -2  2 -2 -2  2  2 -2 12  4  0  0  0  0
J  0 -2  2 -2  2  2 -2 -2  2  4 12  0  0  0  0
K  0  2 -2 -2  2  2 -2  2 -2  0  0 12  4  0  0
L  0 -2  2  2 -2 -2  2 -2  2  0  0  4 12  0  0
M  0 -2  2  2 -2  2 -2  2 -2  0  0  0  0 12  4
N  0  2 -2 -2  2 -2  2 -2  2  0  0  0  0  4 12
\end{verbatim}
\end{multicols}
\end{scriptsize}

\en $d_3$: $(b_1, b_2)=(1/3,2)$ with 11 level-balanced factors
\begin{scriptsize}

\begin{multicols}{2}
\begin{verbatim}


  A  B  C  D  E  F  G  H  I  J  K  L  M  N
  1  1  1  1  1  1  1  1  1  1  1  1  1  1
  1  1  1 -1 -1 -1 -1  1  1  1  1 -1 -1 -1
  1  1  1  1  1  1  1 -1 -1 -1 -1 -1 -1 -1
  1  1  1 -1 -1 -1 -1 -1 -1 -1 -1  1  1  1
 -1  1 -1  1 -1  1 -1 -1 -1  1  1  1 -1  1
 -1  1 -1 -1  1 -1  1 -1 -1  1  1 -1  1 -1
 -1  1 -1  1 -1  1 -1  1  1 -1 -1 -1  1 -1
 -1  1 -1 -1  1 -1  1  1  1 -1 -1  1 -1  1
  1 -1 -1 -1 -1  1  1  1 -1  1 -1  1  1 -1
  1 -1 -1  1  1 -1 -1  1 -1  1 -1 -1 -1  1
  1 -1 -1 -1 -1  1  1 -1  1 -1  1 -1 -1  1
  1 -1 -1  1  1 -1 -1 -1  1 -1  1  1  1 -1



      A  B  C  D  E  F  G  H  I  J  K  L  M  N
  12  4  4 -4  0  0  0  0  0  0  0  0  0  0  0
A  4 12 -4  4  0  0  0  0  0  0  0  0  0  0  0
B  4 -4 12  4  0  0  0  0  0  0  0  0  0  0  0
C -4  4  4 12  0  0  0  0  0  0  0  0  0  0  0
D  0  0  0  0 12  4  4 -4  0  0  0  0  0  0  0
E  0  0  0  0  4 12 -4  4  0  0  0  0  0  0  0
F  0  0  0  0  4 -4 12  4  0  0  0  0  0  0  0
G  0  0  0  0 -4  4  4 12  0  0  0  0  0  0  0
H  0  0  0  0  0  0  0  0 12  4  4 -4  0  0  0
I  0  0  0  0  0  0  0  0  4 12 -4  4  0  0  0
J  0  0  0  0  0  0  0  0  4 -4 12  4  0  0  0
K  0  0  0  0  0  0  0  0 -4  4  4 12  0  0  0
L  0  0  0  0  0  0  0  0  0  0  0  0 12  4  4
M  0  0  0  0  0  0  0  0  0  0  0  0  4 12 -4
N  0  0  0  0  0  0  0  0  0  0  0  0  4 -4 12
\end{verbatim}
\end{multicols}
\end{scriptsize}

\pagebreak

\en $d_4$: $(b_1, b_2)=(2/9,19/9)$ with 12 level-balanced factors

\begin{scriptsize}

\begin{multicols}{2}
\begin{verbatim}

  A  B  C  D  E  F  G  H  I  J  K  L  M  N
  1 -1 -1  1 -1 -1  1  1 -1  1 -1  1  1  1
  1 -1  1  1  1 -1 -1 -1  1 -1 -1 -1  1 -1
  1  1  1  1 -1  1 -1 -1 -1  1 -1 -1 -1  1
 -1  1  1  1  1 -1  1  1 -1  1  1 -1 -1 -1
  1  1 -1 -1  1 -1 -1 -1 -1  1  1  1  1 -1
  1  1  1  1 -1  1  1  1  1 -1  1  1  1 -1
  1  1 -1 -1  1 -1  1  1  1 -1 -1 -1 -1  1
 -1  1  1 -1  1  1  1 -1  1  1 -1  1  1  1
  1 -1  1 -1  1  1 -1  1 -1 -1  1  1 -1  1
 -1  1 -1  1 -1 -1 -1 -1  1 -1  1  1 -1  1
  1 -1 -1 -1 -1  1  1 -1  1  1  1 -1 -1 -1
 -1  1 -1 -1 -1  1 -1  1 -1 -1 -1 -1  1 -1



      A  B  C  D  E  F  G  H  I  J  K  L  M  N
  12  4  4  0  0  0  0  0  0  0  0  0  0  0  0
A  4 12 -4  0  0  0  0  0  0  0  0  0  0  0  0
B  4 -4 12  0  0  0  0  0  0  0  0  0  0  0  0
C  0  0  0 12  4  4  4  0  0  0  0  0  0  0  0
D  0  0  0  4 12 -4 -4  0  0  0  0  0  0  0  0
E  0  0  0  4 -4 12 -4  0  0  0  0  0  0  0  0
F  0  0  0  4 -4 -4 12  0  0  0  0  0  0  0  0
G  0  0  0  0  0  0  0 12  4  4  4  0  0  0  0
H  0  0  0  0  0  0  0  4 12 -4 -4  0  0  0  0
I  0  0  0  0  0  0  0  4 -4 12 -4  0  0  0  0
J  0  0  0  0  0  0  0  4 -4 -4 12  0  0  0  0
K  0  0  0  0  0  0  0  0  0  0  0 12  4 -4 -4
L  0  0  0  0  0  0  0  0  0  0  0  4 12  4  4
M  0  0  0  0  0  0  0  0  0  0  0 -4  4 12 -4
N  0  0  0  0  0  0  0  0  0  0  0 -4  4 -4 12

\end{verbatim}
\end{multicols}
\end{scriptsize}

\en $d_5$: $(b_1, b_2)=(1/3,2)$ with 5 level-balanced factors

\begin{scriptsize}

\begin{multicols}{2}
%\vspace{3cm}
\begin{verbatim}

 A  B  C  D  E  F  G  H  I  J  K  L  M  N
 1 -1  1 -1 -1 -1  1 -1  1 -1  1 -1 -1  1
 1  1 -1  1  1  1  1 -1 -1 -1 -1 -1  1  1
 1 -1  1 -1  1  1 -1  1  1  1 -1 -1  1 -1
 1  1  1  1  1 -1 -1 -1  1 -1  1  1  1 -1
-1  1 -1 -1  1  1  1 -1  1  1  1  1 -1 -1
-1  1  1 -1 -1  1 -1 -1 -1 -1 -1 -1 -1 -1
-1 -1 -1  1 -1  1 -1 -1  1  1  1 -1  1  1
-1  1 -1 -1 -1 -1 -1  1  1 -1 -1  1  1  1
 1 -1 -1 -1 -1  1  1  1 -1 -1  1  1  1 -1
 1  1 -1  1 -1 -1  1  1  1  1 -1 -1 -1 -1
 1  1  1  1 -1  1 -1  1 -1  1  1  1 -1  1
 1 -1 -1 -1  1 -1 -1 -1 -1  1 -1  1 -1  1



     A  B  C  D  E  F  G  H  I  J  K  L  M  N
  12  4  2 -2  2  2 -2  2 -2 -2  0  0  0  0  0
A  4 12 -2  2 -2 -2  2 -2  2  2  0  0  0  0  0
B  2 -2 12  0  0  0  0  0  0  4  2 -2 -2 -2  2
C -2  2  0 12  0  4  0  0  0  0  2 -2  2 -2 -2
D  2 -2  0  0 12  0  0 -4  0  0 -2 -2  2 -2 -2
E  2 -2  0  4  0 12  0  0  0  0 -2  2 -2  2  2
F -2  2  0  0  0  0 12  0 -4  0 -2 -2 -2 -2  2
G  2 -2  0  0 -4  0  0 12  0  0 -2 -2  2 -2 -2
H -2  2  0  0  0  0 -4  0 12  0 -2 -2 -2 -2  2
I -2  2  4  0  0  0  0  0  0 12 -2  2  2  2 -2
J  0  0  2  2 -2 -2 -2 -2 -2 -2 12  0  0  0  0
K  0  0 -2 -2 -2  2 -2 -2 -2  2  0 12  0 -4  0
L  0  0 -2  2  2 -2 -2  2 -2  2  0  0 12  0  4
M  0  0 -2 -2 -2  2 -2 -2 -2  2  0 -4  0 12  0
N  0  0  2 -2 -2  2  2 -2  2 -2  0  0  4  0 12
\end{verbatim}
\end{multicols}
\end{scriptsize}

\ee

\pagebreak

\subsection*{Case 2: $m=9$ and $N=10$}

Saturated main-effect designs with some given patterns for different
ranges of $\pi_1$. For each case, we list two designs: one is
obtained from the modification of a conference matrix and the other is
obtained from our algorithm. The corresponding $X^\top X$ matrices are
also given.
%As discussed in the paper, both methods generate $Q_B$-optimal
%saturated main-effect designs with the correct number of
%level-balanced factors, but designs generated by the exchange
%algorithm have lower $A_s$-efficiencies for the main effect model, as
%given in Table 2 of the paper.

\begin{footnotesize}
\be\itemsep=0pt

\en $\pi\in (0, 1/16]$

 modification of conference matrix
\vspace{-10pt}
\begin{multicols}{2}
\begin{verbatim}
    A  B  C  D  E  F  G  H  I
1   1  1  1  1  1  1  1  1  1
2  -1  1  1 -1 -1  1 -1  1 -1
3   1 -1  1  1 -1 -1 -1 -1  1
4   1  1 -1 -1  1 -1  1 -1 -1
5  -1  1 -1 -1  1  1 -1 -1  1
6  -1 -1  1  1 -1  1  1 -1 -1
7   1 -1 -1  1  1 -1 -1  1 -1
8  -1 -1  1 -1  1 -1 -1  1  1
9   1 -1 -1 -1 -1  1  1 -1  1
10 -1  1 -1  1 -1 -1  1  1 -1

      A  B  C  D  E  F  G  H  I
  10  0  0  0  0  0  0  0  0  0
A  0 10 -2 -2  2  2 -2  2 -2  2
B  0 -2 10 -2 -2  2  2  2  2 -2
C  0 -2 -2 10  2 -2  2 -2  2  2
D  0  2 -2  2 10 -2 -2  2  2 -2
E  0  2  2 -2 -2 10 -2 -2  2  2
F  0 -2  2  2 -2 -2 10  2 -2  2
G  0  2  2 -2  2 -2  2 10 -2 -2
H  0 -2  2  2  2  2 -2 -2 10 -2
I  0  2 -2  2 -2  2  2 -2 -2 10
\end{verbatim}
\end{multicols}
\vspace{-20pt}
algorithm
\vspace{-10pt}
\begin{multicols}{2}
\begin{verbatim}
    A  B  C  D  E  F  G  H  I
1   1 -1 -1 -1  1 -1  1  1  1
2   1  1  1  1  1 -1 -1 -1 -1
3   1  1  1 -1 -1 -1 -1  1  1
4  -1 -1  1 -1  1 -1 -1 -1  1
5  -1 -1 -1  1 -1 -1  1  1 -1
6   1 -1 -1 -1 -1  1 -1  1 -1
7  -1  1  1  1  1  1  1  1 -1
8   1 -1  1  1 -1  1  1 -1  1
9  -1  1 -1  1  1  1 -1 -1  1
10 -1  1 -1 -1 -1  1  1 -1 -1

      A  B  C  D  E  F  G  H  I
  10  0  0  0  0  0  0  0  0  0
A  0 10 -2  2 -2 -2 -2 -2  2  2
B  0 -2 10  2  2  2  2 -2 -2 -2
C  0  2  2 10  2  2 -2 -2 -2  2
D  0 -2  2  2 10  2  2  2 -2 -2
E  0 -2  2  2  2 10 -2 -2 -2  2
F  0 -2  2 -2  2 -2 10  2 -2 -2
G  0 -2 -2 -2  2 -2  2 10  2 -2
H  0  2 -2 -2 -2 -2 -2  2 10 -2
I  0  2 -2  2 -2  2 -2 -2 -2 10
\end{verbatim}
\end{multicols}
\en $\pi\in (1/16, 1/12]$
  
 modification of conference matrix
 \vspace{-10pt}
\begin{multicols}{2}
\begin{verbatim}

    A  B  C  D  E  F  G  H  I
1   1  1  1  1  1  1  1  1  1
2  -1 -1  1  1 -1 -1  1 -1  1
3   1  1 -1  1  1 -1 -1 -1 -1
4  -1  1  1 -1 -1  1 -1  1 -1
5   1 -1  1 -1 -1  1  1 -1 -1
6  -1 -1 -1  1  1 -1  1  1 -1
7  -1  1 -1 -1  1  1 -1 -1  1
8   1 -1 -1  1 -1  1 -1 -1  1
9   1  1 -1 -1 -1 -1  1  1 -1
10  1 -1  1 -1  1 -1 -1  1  1

      A  B  C  D  E  F  G  H  I
  10  2  0  0  0  0  0  0  0  0
A  2 10  0  0  0  0  0  0  0  0
B  0  0 10 -2 -2  2  2 -2  2 -2
C  0  0 -2 10 -2 -2  2  2  2  2
D  0  0 -2 -2 10  2 -2  2 -2  2
E  0  0  2 -2  2 10 -2 -2  2  2
F  0  0  2  2 -2 -2 10 -2 -2  2
G  0  0 -2  2  2 -2 -2 10  2 -2
H  0  0  2  2 -2  2 -2  2 10 -2
I  0  0 -2  2  2  2  2 -2 -2 10
\end{verbatim}
\end{multicols}
\vspace{-10pt}

%\pagebreak

algorithm
\vspace{-20pt}
\begin{multicols}{2}
\begin{verbatim}

    A  B  C  D  E  F  G  H  I
1  -1 -1 -1 -1  1  1  1 -1 -1
2  -1 -1  1  1 -1 -1  1  1 -1
3   1 -1  1  1  1 -1 -1 -1 -1
4   1  1  1 -1  1  1  1  1 -1
5  -1  1 -1 -1  1 -1 -1  1  1
6   1 -1 -1  1  1  1  1  1  1
7   1 -1 -1 -1 -1  1 -1  1  1
8  -1  1  1  1 -1  1 -1 -1  1
9   1  1 -1  1 -1 -1 -1 -1 -1
10  1  1  1 -1 -1 -1  1 -1  1

      A  B  C  D  E  F  G  H  I
  10  2  0  0  0  0  0  0  0  0
A  2 10  0  0  0  0  0  0  0  0
B  0  0 10  2 -2 -2 -2 -2 -2  2
C  0  0  2 10  2 -2 -2  2 -2 -2
D  0  0 -2  2 10 -2 -2 -2 -2 -2
E  0  0 -2 -2 -2 10  2  2  2 -2
F  0  0 -2 -2 -2  2 10  2  2  2
G  0  0 -2  2 -2  2  2 10  2 -2
H  0  0 -2 -2 -2  2  2  2 10  2
I  0  0  2 -2 -2 -2  2 -2  2 10
\end{verbatim}
\end{multicols}

\en $\pi\in (1/12, 1/8]$
  
 modification of conference matrix
% we found saturated main-effect design with 7 level-balanced factors by both methods.
\vspace{-20pt}
\begin{multicols}{2}
\begin{verbatim}

    A  B  C  D  E  F  G  H  I
1   1  1  1  1  1  1  1  1  1
2   1 -1  1  1 -1 -1  1 -1  1
3   1  1 -1  1  1 -1 -1 -1 -1
4   1 -1  1 -1 -1  1 -1  1 -1
5  -1  1  1 -1 -1  1  1 -1 -1
6  -1 -1 -1  1  1 -1  1  1 -1
7   1 -1 -1 -1  1  1 -1 -1  1
8  -1  1 -1  1 -1  1 -1 -1  1
9   1  1 -1 -1 -1 -1  1  1 -1
10 -1  1  1 -1  1 -1 -1  1  1

      A  B  C  D  E  F  G  H  I
  10  2  2  0  0  0  0  0  0  0
A  2 10 -2  0  0  0  0  0  0  0
B  2 -2 10  0  0  0  0  0  0  0
C  0  0  0 10 -2 -2  2  2  2  2
D  0  0  0 -2 10  2 -2  2 -2  2
E  0  0  0 -2  2 10 -2 -2  2  2
F  0  0  0  2 -2 -2 10 -2 -2  2
G  0  0  0  2  2 -2 -2 10  2 -2
H  0  0  0  2 -2  2 -2  2 10 -2
I  0  0  0  2  2  2  2 -2 -2 10
\end{verbatim}
\end{multicols}
\vspace{-10pt}
algorithm
\vspace{-20pt}
\begin{multicols}{2}
\begin{verbatim}

    A  B  C  D  E  F  G  H  I
1   1 -1 -1  1  1  1 -1 -1 -1
2   1  1 -1 -1 -1 -1  1 -1  1
3  -1  1  1 -1  1 -1 -1 -1 -1
4   1 -1  1 -1  1 -1  1  1  1
5  -1 -1  1 -1 -1  1  1  1 -1
6   1  1  1  1 -1  1 -1  1 -1
7  -1  1  1  1  1  1  1 -1  1
8  -1  1 -1  1  1 -1  1  1 -1
9  -1 -1 -1  1 -1 -1 -1 -1  1
10 -1  1 -1 -1 -1  1 -1  1  1

      A  B  C  D  E  F  G  H  I
  10 -2  2  0  0  0  0  0  0  0
A -2 10 -2  0  0  0  0  0  0  0
B  2 -2 10  0  0  0  0  0  0  0
C  0  0  0 10 -2  2  2  2  2 -2
D  0  0  0 -2 10  2  2 -2 -2 -2
E  0  0  0  2  2 10 -2  2 -2 -2
F  0  0  0  2  2 -2 10 -2  2 -2
G  0  0  0  2 -2  2 -2 10  2  2
H  0  0  0  2 -2 -2  2  2 10 -2
I  0  0  0 -2 -2 -2 -2  2 -2 10
\end{verbatim}
\end{multicols}

\en $\pi\in (1/8, 1/4]$

 modification of conference matrix
\vspace{-10pt}
\begin{multicols}{2}
\begin{verbatim}

    A  B  C  D  E  F  G  H  I
1   1  1  1  1  1  1  1  1  1
2   1  1 -1  1  1 -1 -1  1 -1
3   1 -1  1 -1  1  1 -1 -1 -1
4   1 -1 -1  1 -1 -1  1 -1  1
5  -1 -1  1  1 -1 -1  1  1 -1
6  -1 -1 -1 -1  1  1 -1  1  1
7   1  1 -1 -1 -1  1  1 -1 -1
8  -1  1  1 -1  1 -1  1 -1 -1
9   1  1  1 -1 -1 -1 -1  1  1
10 -1  1  1  1 -1  1 -1 -1  1

      A  B  C  D  E  F  G  H  I
  10  2  2  2  0  0  0  0  0  0
A  2 10  2 -2  0  0  0  0  0  0
B  2  2 10  2  0  0  0  0  0  0
C  2 -2  2 10  0  0  0  0  0  0
D  0  0  0  0 10 -2 -2  2  2  2
E  0  0  0  0 -2 10  2 -2  2 -2
F  0  0  0  0 -2  2 10 -2 -2  2
G  0  0  0  0  2 -2 -2 10 -2 -2
H  0  0  0  0  2  2 -2 -2 10  2
I  0  0  0  0  2 -2  2 -2  2 10
\end{verbatim}
\end{multicols}
\vspace{-10pt}
algorithm
\vspace{-10pt}
\begin{multicols}{2}
\begin{verbatim}
    A  B  C  D  E  F  G  H  I
1   1 -1 -1  1 -1  1 -1 -1 -1
2   1 -1 -1 -1  1  1  1  1 -1
3   1  1  1 -1 -1 -1  1 -1  1
4   1 -1 -1 -1 -1 -1 -1  1  1
5  -1  1 -1 -1  1 -1 -1 -1 -1
6   1  1  1  1  1  1 -1  1 -1
7  -1  1 -1  1 -1  1  1  1  1
8  -1 -1  1 -1  1  1 -1 -1  1
9   1 -1 -1  1  1 -1  1 -1  1
10 -1 -1  1  1 -1 -1  1  1 -1

      A  B  C  D  E  F  G  H  I
  10  2 -2 -2  0  0  0  0  0  0
A  2 10 -2 -2  0  0  0  0  0  0
B -2 -2 10  2  0  0  0  0  0  0
C -2 -2  2 10  0  0  0  0  0  0
D  0  0  0  0 10 -2  2  2  2 -2
E  0  0  0  0 -2 10  2 -2 -2 -2
F  0  0  0  0  2  2 10 -2  2 -2
G  0  0  0  0  2 -2 -2 10  2  2
H  0  0  0  0  2 -2  2  2 10 -2
I  0  0  0  0 -2 -2 -2  2 -2 10
\end{verbatim}
\end{multicols}
\vspace{-10pt}

\pagebreak

\en $\pi\in (1/4, 1]$
  modification of conference matrix
  
\vspace{-10pt}
\begin{multicols}{2}
\begin{verbatim}

    A  B  C  D  E  F  G  H  I
1   1  1  1  1  1  1  1  1  1
2   1 -1  1 -1  1  1 -1 -1  1
3   1  1 -1  1 -1  1 -1 -1 -1
4   1 -1 -1 -1  1 -1  1  1 -1
5  -1  1  1  1  1 -1  1 -1 -1
6  -1  1  1 -1 -1  1 -1  1 -1
7   1  1  1 -1 -1 -1  1 -1  1
8  -1 -1 -1  1 -1  1  1 -1  1
9   1 -1  1  1 -1 -1 -1  1 -1
10 -1  1 -1  1  1 -1 -1  1  1

      A  B  C  D  E  F  G  H  I
  10  2  2  2  2  0  0  0  0  0
A  2 10 -2  2 -2  0  0  0  0  0
B  2 -2 10  2  2  0  0  0  0  0
C  2  2  2 10 -2  0  0  0  0  0
D  2 -2  2 -2 10  0  0  0  0  0
E  0  0  0  0  0 10 -2  2  2  2
F  0  0  0  0  0 -2 10 -2 -2  2
G  0  0  0  0  0  2 -2 10 -2  2
H  0  0  0  0  0  2 -2 -2 10 -2
I  0  0  0  0  0  2  2  2 -2 10
\end{verbatim}
\end{multicols}
\vspace{-10pt}
algorithm
\vspace{-10pt}
\begin{multicols}{2}
\begin{verbatim}

    A  B  C  D  E  F  G  H  I
1  -1  1 -1  1  1 -1  1 -1  1
2   1  1 -1 -1  1  1  1  1  1
3  -1  1 -1  1 -1  1 -1  1 -1
4  -1  1  1 -1  1  1 -1 -1 -1
5  -1 -1 -1 -1 -1  1 -1 -1  1
6  -1  1  1 -1 -1 -1  1  1  1
7   1  1 -1 -1 -1 -1 -1 -1 -1
8   1 -1  1  1  1 -1 -1  1  1
9   1 -1  1  1 -1  1  1 -1 -1
10 -1 -1 -1 -1  1 -1  1  1 -1

      A  B  C  D  E  F  G  H  I
  10 -2  2 -2 -2  0  0  0  0  0
A -2 10 -2  2  2  0  0  0  0  0
B  2 -2 10 -2 -2  0  0  0  0  0
C -2  2 -2 10  2  0  0  0  0  0
D -2  2 -2  2 10  0  0  0  0  0
E  0  0  0  0  0 10 -2  2  2  2
F  0  0  0  0  0 -2 10 -2 -2 -2
G  0  0  0  0  0  2 -2 10  2  2
H  0  0  0  0  0  2 -2  2 10  2
I  0  0  0  0  0  2 -2  2  2 10
\end{verbatim}
\end{multicols}
\ee
\end{footnotesize}

 \subsubsection*{Case 3:  \(m=12\) and \(N=14\)}
 Designs and information matrices for \(m=12\) and \(N=14\) under different $\pi_1$. 

 \begin{footnotesize}
\be\itemsep=0pt
\en $\pi_1\in (0, 1/22]$
\begin{multicols}{2}
\begin{verbatim}
    A  B  C  D  E  F  G  H  I  J
1   1 -1 -1 -1  1 -1  1 -1  1 -1
2  -1 -1  1 -1 -1  1 -1  1  1 -1
3  -1 -1 -1 -1 -1  1 -1  1 -1  1
4  -1  1 -1 -1  1 -1  1  1 -1  1
5   1  1  1 -1 -1 -1  1 -1 -1  1
6   1 -1 -1  1 -1  1  1 -1  1  1
7  -1  1  1 -1  1  1 -1 -1 -1 -1
8  -1  1 -1  1 -1 -1 -1 -1 -1 -1
9  -1 -1  1  1 -1 -1  1  1  1 -1
10  1  1 -1  1  1 -1 -1  1  1  1
11  1 -1  1  1  1 -1 -1 -1 -1  1
12  1 -1 -1  1  1  1  1  1 -1 -1
13 -1  1  1  1  1  1  1 -1  1  1
14  1  1  1 -1 -1  1 -1  1  1 -1


      A  B  C  D  E  F  G  H  I  J
  14  0  0  0  0  0  0  0  0  0  0
A  0 14 -2 -2  2  2 -2  2 -2  2  2
B  0 -2 14  2 -2  2 -2 -2 -2 -2  2
C  0 -2  2 14 -2 -2  2 -2 -2  2 -2
D  0  2 -2 -2 14  2 -2  2 -2  2  2
E  0  2  2 -2  2 14 -2  2 -2 -2  2
F  0 -2 -2  2 -2 -2 14 -2  2  2 -2
G  0  2 -2 -2  2  2 -2 14 -2  2  2
H  0 -2 -2 -2 -2 -2  2 -2 14  2 -2
I  0  2 -2  2  2 -2  2  2  2 14 -2
J  0  2  2 -2  2  2 -2  2 -2 -2 14


\end{verbatim}
\end{multicols}

\pagebreak

\en $\pi_1\in (1/22, 1/18]$
\begin{multicols}{2}
\begin{verbatim}
    A  B  C  D  E  F  G  H  I  J
1   1 -1  1 -1  1 -1  1 -1  1 -1
2   1  1 -1  1  1  1  1 -1  1  1
3   1 -1 -1  1  1 -1 -1  1  1 -1
4  -1 -1 -1 -1 -1  1 -1 -1  1 -1
5  -1  1  1  1  1  1 -1 -1  1  1
6   1 -1 -1 -1 -1  1 -1  1 -1 -1
7  -1 -1  1 -1  1 -1 -1  1 -1  1
8   1  1  1 -1 -1 -1 -1  1 -1  1
9  -1  1 -1 -1 -1 -1  1  1  1 -1
10  1  1 -1 -1  1  1  1 -1 -1  1
11 -1 -1 -1  1 -1 -1  1 -1 -1  1
12  1 -1  1  1 -1  1  1  1  1  1
13  1  1  1  1 -1 -1 -1 -1 -1 -1
14 -1  1  1  1  1  1  1  1 -1 -1

      A  B  C  D  E  F  G  H  I  J
  14  2  0  0  0  0  0  0  0  0  0
A  2 14  0  0  0  0  0  0  0  0  0
B  0  0 14  2  2  2  2  2 -2 -2  2
C  0  0  2 14  2  2 -2 -2  2 -2  2
D  0  0  2  2 14  2  2  2 -2  2  2
E  0  0  2  2  2 14  2  2 -2  2  2
F  0  0  2 -2  2  2 14  2 -2  2  2
G  0  0  2 -2  2  2  2 14 -2  2  2
H  0  0 -2  2 -2 -2 -2 -2 14 -2 -2
I  0  0 -2 -2  2  2  2  2 -2 14 -2
J  0  0  2  2  2  2  2  2 -2 -2 14


\end{verbatim}
\end{multicols}

\vspace{-10pt}
\en $\pi_1\in (1/18, 1/14]$
\begin{multicols}{2}
\begin{verbatim}
    A  B  C  D  E  F  G  H  I  J
1   1  1  1 -1  1 -1 -1  1 -1  1
2   1 -1 -1 -1 -1 -1  1  1 -1 -1
3  -1  1 -1 -1  1  1  1 -1 -1  1
4   1  1 -1  1  1  1 -1  1  1 -1
5  -1  1 -1 -1 -1 -1 -1 -1  1 -1
6  -1  1 -1  1 -1  1  1  1 -1 -1
7   1 -1 -1  1  1 -1  1 -1  1  1
8  -1  1  1  1  1 -1 -1  1 -1  1
9  -1 -1 -1 -1 -1  1 -1  1  1  1
10 -1  1  1  1 -1 -1  1 -1  1  1
11  1  1  1 -1 -1  1  1 -1  1 -1
12 -1 -1  1  1  1 -1 -1 -1 -1 -1
13 -1 -1  1 -1  1  1  1  1  1 -1
14  1 -1  1  1 -1  1 -1 -1 -1  1

      A  B  C  D  E  F  G  H  I  J
  14 -2  2  0  0  0  0  0  0  0  0
A -2 14 -2  0  0  0  0  0  0  0  0
B  2 -2 14  0  0  0  0  0  0  0  0
C  0  0  0 14  2  2 -2 -2 -2 -2  2
D  0  0  0  2 14  2 -2 -2 -2 -2  2
E  0  0  0  2  2 14 -2 -2  2 -2  2
F  0  0  0 -2 -2 -2 14  2  2  2 -2
G  0  0  0 -2 -2 -2  2 14 -2  2 -2
H  0  0  0 -2 -2  2  2 -2 14 -2 -2
I  0  0  0 -2 -2 -2  2  2 -2 14 -2
J  0  0  0  2  2  2 -2 -2 -2 -2 14


\end{verbatim}
\end{multicols}
\vspace{-10pt}
\en $\pi_1\in (1/14, 1/10]$
\begin{multicols}{2}
\begin{verbatim}
    A  B  C  D  E  F  G  H  I  J
1  -1  1 -1  1  1 -1  1  1  1 -1
2  -1 -1  1 -1  1 -1  1  1 -1  1
3   1 -1  1  1  1  1  1 -1  1  1
4  -1  1  1 -1 -1  1  1  1  1  1
5   1  1 -1 -1  1  1 -1 -1  1 -1
6   1 -1  1  1 -1 -1 -1  1  1 -1
7  -1 -1 -1  1 -1  1  1 -1 -1 -1
8   1  1  1 -1 -1 -1  1 -1 -1 -1
9  -1 -1  1 -1  1  1 -1  1 -1 -1
10  1  1 -1 -1  1 -1  1  1 -1  1
11  1  1 -1  1 -1  1 -1  1 -1  1
12 -1  1  1  1 -1  1 -1 -1  1 -1
13 -1  1  1  1  1 -1 -1 -1 -1  1
14 -1 -1 -1 -1 -1 -1 -1 -1  1  1

      A  B  C  D  E  F  G  H  I  J
  14 -2  2  2  0  0  0  0  0  0  0
A -2 14  2 -2  0  0  0  0  0  0  0
B  2  2 14 -2  0  0  0  0  0  0  0
C  2 -2 -2 14  0  0  0  0  0  0  0
D  0  0  0  0 14 -2  2 -2 -2  2 -2
E  0  0  0  0 -2 14 -2  2  2 -2  2
F  0  0  0  0  2 -2 14 -2 -2  2 -2
G  0  0  0  0 -2  2 -2 14  2 -2  2
H  0  0  0  0 -2  2 -2  2 14 -2  2
I  0  0  0  0  2 -2  2 -2 -2 14 -2
J  0  0  0  0 -2  2 -2  2  2 -2 14


\end{verbatim}
\end{multicols}
\pagebreak

\vspace{-10pt}
\en $\pi_1\in (1/10,1/6]$
\begin{multicols}{2}
\begin{verbatim}
    A  B  C  D  E  F  G  H  I  J
1  -1  1 -1 -1 -1 -1  1 -1  1 -1
2  -1  1  1  1 -1  1 -1  1 -1  1
3   1  1  1 -1  1  1  1  1  1  1
4   1 -1 -1 -1  1 -1 -1  1 -1  1
5   1  1  1  1  1 -1 -1 -1  1  1
6   1  1 -1  1  1  1 -1 -1 -1 -1
7  -1  1 -1  1  1 -1  1  1 -1  1
8   1  1  1 -1 -1  1  1 -1 -1 -1
9   1 -1 -1  1 -1  1  1  1  1 -1
10  1 -1  1  1 -1 -1  1 -1 -1  1
11 -1 -1  1 -1  1 -1 -1  1 -1 -1
12 -1 -1  1  1  1  1  1 -1  1 -1
13 -1 -1 -1 -1 -1  1 -1 -1  1  1
14  1  1  1  1 -1 -1 -1  1  1 -1

      A  B  C  D  E  F  G  H  I  J
  14  2  2  2  2  0  0  0  0  0  0
A  2 14  2  2  2  0  0  0  0  0  0
B  2  2 14  2  2  0  0  0  0  0  0
C  2  2  2 14  2  0  0  0  0  0  0
D  2  2  2  2 14  0  0  0  0  0  0
E  0  0  0  0  0 14 -2 -2  2 -2  2
F  0  0  0  0  0 -2 14  2 -2  2 -2
G  0  0  0  0  0 -2  2 14 -2  2 -2
H  0  0  0  0  0  2 -2 -2 14 -2  2
I  0  0  0  0  0 -2  2  2 -2 14 -2
J  0  0  0  0  0  2 -2 -2  2 -2 14


\end{verbatim}
\end{multicols}
\vspace{-10pt}
\en $\pi_1\in (1/6,1/2]$
\begin{multicols}{2}
\begin{verbatim}
    A  B  C  D  E  F  G  H  I  J
1   1 -1  1 -1 -1  1  1  1  1  1
2   1 -1 -1  1 -1 -1  1  1 -1 -1
3   1  1  1  1  1 -1  1  1  1  1
4  -1 -1  1 -1  1 -1 -1  1 -1  1
5  -1  1 -1  1 -1 -1 -1  1  1  1
6  -1 -1 -1 -1  1 -1  1 -1  1  1
7  -1  1  1 -1 -1 -1  1 -1 -1 -1
8  -1  1  1 -1  1  1 -1  1 -1 -1
9  -1  1 -1 -1  1  1  1  1  1 -1
10  1  1  1 -1  1 -1 -1 -1  1 -1
11 -1 -1  1  1 -1  1 -1 -1  1 -1
12  1  1 -1 -1 -1  1 -1 -1 -1  1
13 -1  1  1  1  1  1  1 -1 -1  1
14  1 -1 -1  1  1  1 -1 -1 -1 -1

      A  B  C  D  E  F  G  H  I  J
  14 -2  2  2 -2  2  0  0  0  0  0
A -2 14 -2 -2  2 -2  0  0  0  0  0
B  2 -2 14  2 -2  2  0  0  0  0  0
C  2 -2  2 14 -2  2  0  0  0  0  0
D -2  2 -2 -2 14 -2  0  0  0  0  0
E  2 -2  2  2 -2 14  0  0  0  0  0
F  0  0  0  0  0  0 14 -2 -2 -2 -2
G  0  0  0  0  0  0 -2 14  2  2  2
H  0  0  0  0  0  0 -2  2 14  2  2
I  0  0  0  0  0  0 -2  2  2 14  2
J  0  0  0  0  0  0 -2  2  2  2 14


\end{verbatim}
\end{multicols}
\ee
\end{footnotesize}

\(N=22\) and \(m=15\)
  %\begin{multicols}{1}

$\pi_1=0.2$
\begin{footnotesize}
\begin{verbatim}
      A  B  C  D  E  F  G  H  I  J  K  L  M  N  O
  22  2  2 -2  2  2 -2  0  0  0  0  0  0  0  0  0
A  2 22 -2 -2  2  2 -2  0  0  0  0  0  0  0  0  0
B  2 -2 22  2  2  2  2  0  0  0  0  0  0  0  0  0
C -2 -2  2 22  2 -2 -2  0  0  0  0  0  0  0  0  0
D  2  2  2  2 22 -2 -2  0  0  0  0  0  0  0  0  0
E  2  2  2 -2 -2 22  2  0  0  0  0  0  0  0  0  0
F -2 -2  2 -2 -2  2 22  0  0  0  0  0  0  0  0  0
G  0  0  0  0  0  0  0 22 -2  2  2  2  2  2  2 -2
H  0  0  0  0  0  0  0 -2 22  2  2 -2 -2  2  2  2
I  0  0  0  0  0  0  0  2  2 22  2 -2  2  2  2  2
J  0  0  0  0  0  0  0  2  2  2 22  2  2 -2 -2 -2
K  0  0  0  0  0  0  0  2 -2 -2  2 22 -2  2  2  2
L  0  0  0  0  0  0  0  2 -2  2  2 -2 22 -2  2 -2
M  0  0  0  0  0  0  0  2  2  2 -2  2 -2 22 -2  2
N  0  0  0  0  0  0  0  2  2  2 -2  2  2 -2 22  2
O  0  0  0  0  0  0  0 -2  2  2 -2  2 -2  2  2 22

\end{verbatim}

\pagebreak

$\pi_1=0.02$
\begin{verbatim}

      A  B  C  D  E  F  G  H  I  J  K  L  M  N  O
  22  0  0  0  0  0  0  0  0  0  0  0  0  0  0  0
A  0 22  2  2 -2  2  2  2 -2 -2 -2  2 -2 -2  2 -2
B  0  2 22  2 -2 -2  6 -2  2 -2  2 -2 -2 -2 -2  2
C  0  2  2 22  2 -2  2 -2 -2  2 -2  2  2 -2 -2 -2
D  0 -2 -2  2 22 -2 -2  6 -6  2  2 -2  2 -2  2 -2
E  0  2 -2 -2 -2 22  2  2  2  2 -2  2  2 -2  2  2
F  0  2  6  2 -2  2 22 -2 -2 -2  2  2  2 -2  2 -2
G  0  2 -2 -2  6  2 -2 22 -6  2  2  2  2 -2 -2  2
H  0 -2  2 -2 -6  2 -2 -6 22 -2  2  2  2 -2 -2 -2
I  0 -2 -2  2  2  2 -2  2 -2 22 -2  2 -2 -2 -2  2
J  0 -2  2 -2  2 -2  2  2  2 -2 22 -2 -2  2  2 -2
K  0  2 -2  2 -2  2  2  2  2  2 -2 22  2  2 -2  2
L  0 -2 -2  2  2  2  2  2  2 -2 -2  2 22 -2  2  2
M  0 -2 -2 -2 -2 -2 -2 -2 -2 -2  2  2 -2 22 -2  2
N  0  2 -2 -2  2  2  2 -2 -2 -2  2 -2  2 -2 22  2
O  0 -2  2 -2 -2  2 -2  2 -2  2 -2  2  2  2  2 22

\end{verbatim}
%\end{multicols}
\end{footnotesize}

\pagebreak

\subsubsection*{Case 4: \(N=16\)
  and \(m=6\)}

Second-order orthogonal main effect designs with \(N=16\)
and \(m=6\).  The indices of the columns for five $m=6$ designs from the
projection of the Hadamard matrix are (1 2 4 8 11 13), (1 2 4 6 8
11), (1 2 3 4 8 13), (1 2 4 6 8 9), and (1 2 3 4 8 12), respectively,
where only two designs are admissible, denoted as $d_1$ and $d_3$ in
Table 5 of the paper.  We give the above two designs and a design
$d_6$ generated by the algorithm and the  information
matrices for the second-order model of these three designs are also given.  

\begin{small}
%\begin{table}[ht]
\begin{center}
Hadamard matrix of order 16
\end{center}
%\label{tab:had16}
%{\footnotesize
\begin{center}
\renewcommand{\arraystretch}{.6}\addtolength{\tabcolsep}{0pt}
\begin{tabular}{*{16}{r}}
 & 1 & 2 & 3 & 4 & 5 & 6 & 7 & 8 & 9 & 10 & 11 & 12 & 13 & 14 & 15 \\ 
 \hline
 1 & 1 & 1 & 1 & 1 & 1 & 1 & 1 & 1 & 1 & 1 & 1 & 1 & 1 & 1 & 1 \\ 
 2 & -1 & 1 & -1 & 1 & -1 & 1 & -1 & 1 & -1 & 1 & -1 & 1 & -1 & 1 & -1 \\ 
 3 & 1 & -1 & -1 & 1 & 1 & -1 & -1 & 1 & 1 & -1 & -1 & 1 & 1 & -1 & -1 \\ 
 4 & -1 & -1 & 1 & 1 & -1 & -1 & 1 & 1 & -1 & -1 & 1 & 1 & -1 & -1 & 1 \\ 
 5 & 1 & 1 & 1 & -1 & -1 & -1 & -1 & 1 & 1 & 1 & 1 & -1 & -1 & -1 & -1 \\ 
 6 & -1 & 1 & -1 & -1 & 1 & -1 & 1 & 1 & -1 & 1 & -1 & -1 & 1 & -1 & 1 \\ 
 7 & 1 & -1 & -1 & -1 & -1 & 1 & 1 & 1 & 1 & -1 & -1 & -1 & -1 & 1 & 1 \\ 
 8 & -1 & -1 & 1 & -1 & 1 & 1 & -1 & 1 & -1 & -1 & 1 & -1 & 1 & 1 & -1 \\ 
 9 & 1 & 1 & 1 & 1 & 1 & 1 & 1 & -1 & -1 & -1 & -1 & -1 & -1 & -1 & -1 \\ 
 10 & -1 & 1 & -1 & 1 & -1 & -1 & 1 & -1 & 1 & -1 & 1 & -1 & 1 & 1 & -1 \\ 
 11 & 1 & -1 & -1 & 1 & 1 & -1 & -1 & -1 & -1 & 1 & 1 & -1 & -1 & 1 & 1 \\ 
 12 & -1 & -1 & 1 & 1 & -1 & 1 & -1 & -1 & 1 & 1 & -1 & -1 & 1 & -1 & 1 \\ 
 13 & 1 & 1 & 1 & -1 & -1 & -1 & -1 & -1 & -1 & -1 & -1 & 1 & 1 & 1 & 1 \\ 
 14 & -1 & 1 & -1 & -1 & 1 & 1 & -1 & -1 & 1 & -1 & 1 & 1 & -1 & -1 & 1 \\ 
 15 & 1 & -1 & -1 & -1 & -1 & 1 & 1 & -1 & -1 & 1 & 1 & 1 & 1 & -1 & -1 \\ 
 16 & -1 & -1 & 1 & -1 & 1 & -1 & 1 & -1 & 1 & 1 & -1 & 1 & -1 & 1 & -1 \\ 
 \hline
 \end{tabular}
\end{center}%}
%\end{table}

~ 
%\begin{table}[htp]
%\caption{Three second-order orthogonal main effect designs with $m=6$, $N=16$}
%\label{tab:D2nd16}

%\begin{multicols}{3}%\setlength{\columnsep}{0.5cm}
\begin{center}
    
\renewcommand{\arraystretch}{.8}\addtolength{\tabcolsep}{0pt}
 \begin{tabular}{*{6}{r}}
 \multicolumn{6}{c}{$d_1$}\\
x1 & x2 & x3 & x4 & x5 & x6 \\ \hline
1 & 1 & 1 & 1 & 1 & 1 \\ 
 -1 & 1 & 1 & 1 & -1 & -1 \\ 
 1 & -1 & 1 & 1 & -1 & 1 \\ 
 -1 & -1 & 1 & 1 & 1 & -1 \\ 
 1 & 1 & -1 & 1 & 1 & -1 \\ 
 -1 & 1 & -1 & 1 & -1 & 1 \\ 
 1 & -1 & -1 & 1 & -1 & -1 \\ 
 -1 & -1 & -1 & 1 & 1 & 1 \\ 
 1 & 1 & 1 & -1 & -1 & -1 \\ 
 -1 & 1 & 1 & -1 & 1 & 1 \\ 
 1 & -1 & 1 & -1 & 1 & -1 \\ 
 -1 & -1 & 1 & -1 & -1 & 1 \\ 
 1 & 1 & -1 & -1 & -1 & 1 \\ 
 -1 & 1 & -1 & -1 & 1 & -1 \\ 
 1 & -1 & -1 & -1 & 1 & 1 \\ 
 -1 & -1 & -1 & -1 & -1 & -1 \\\hline 
\end{tabular}
\;
 \begin{tabular}{*{6}{r}}
 \multicolumn{6}{c}{$d_3$}\\
x1 & x2 & x3 & x4 & x5 & x6 \\ \hline
1 & 1 & 1 & 1 & 1 & 1 \\ 
 -1 & 1 & -1 & 1 & 1 & -1 \\ 
 1 & -1 & -1 & 1 & 1 & 1 \\ 
 -1 & -1 & 1 & 1 & 1 & -1 \\ 
 1 & 1 & 1 & -1 & 1 & -1 \\ 
 -1 & 1 & -1 & -1 & 1 & 1 \\ 
 1 & -1 & -1 & -1 & 1 & -1 \\ 
 -1 & -1 & 1 & -1 & 1 & 1 \\ 
 1 & 1 & 1 & 1 & -1 & -1 \\ 
 -1 & 1 & -1 & 1 & -1 & 1 \\ 
 1 & -1 & -1 & 1 & -1 & -1 \\ 
 -1 & -1 & 1 & 1 & -1 & 1 \\ 
 1 & 1 & 1 & -1 & -1 & 1 \\ 
 -1 & 1 & -1 & -1 & -1 & -1 \\ 
 1 & -1 & -1 & -1 & -1 & 1 \\ 
 -1 & -1 & 1 & -1 & -1 & -1 \\ \hline
\end{tabular}
\;
 \begin{tabular}{*{6}{r}}
 \multicolumn{6}{c}{$d_6$}\\
 x1 & x2 & x3 & x4 & x5 & x6 \\ \hline
1 & 1 & -1 & 1 & -1 & 1 \\ 
 -1 & 1 & -1 & 1 & -1 & -1 \\ 
 1 & 1 & 1 & 1 & 1 & -1 \\ 
 -1 & -1 & -1 & -1 & 1 & -1 \\ 
 -1 & -1 & 1 & -1 & 1 & 1 \\ 
 -1 & -1 & -1 & 1 & -1 & 1 \\ 
 1 & -1 & -1 & -1 & -1 & 1 \\ 
 1 & 1 & -1 & -1 & 1 & -1 \\ 
 -1 & 1 & -1 & -1 & 1 & 1 \\ 
 -1 & 1 & 1 & -1 & -1 & -1 \\ 
 -1 & 1 & 1 & 1 & 1 & 1 \\ 
 -1 & -1 & 1 & 1 & -1 & -1 \\ 
 1 & -1 & 1 & -1 & -1 & -1 \\ 
 1 & -1 & 1 & 1 & 1 & 1 \\ 
 1 & 1 & 1 & -1 & -1 & 1 \\ 
 1 & -1 & -1 & 1 & 1 & -1 \\ \hline
\end{tabular}
\end{center}

%\end{multicols}
%\end{table}

%\begin{footnotesize}

\pagebreak

\begin{verbatim}

       A  B  C  D  E  F AB AC AD AE AF BC BD BE BF CD CE CF DE DF EF
   16  0  0  0  0  0  0  0  0  0  0  0  0  0  0  0  0  0  0  0  0  0
A   0 16  0  0  0  0  0  0  0  0  0  0  0  0  0  0  0  0  0  0  0  0
B   0  0 16  0  0  0  0  0  0  0  0  0  0  0  0  0  0  0  0  0  0  0
C   0  0  0 16  0  0  0  0  0  0  0  0  0  0  0  0  0  0  0  0  0  0
D   0  0  0  0 16  0  0  0  0  0  0  0  0  0  0  0  0  0  0  0  0  0
E   0  0  0  0  0 16  0  0  0  0  0  0  0  0  0  0  0  0  0  0  0  0
F   0  0  0  0  0  0 16  0  0  0  0  0  0  0  0  0  0  0  0  0  0  0
AB  0  0  0  0  0  0  0 16  0  0  0  0  0  0  0  0  0  0  0 16  0  0
AC  0  0  0  0  0  0  0  0 16  0  0  0  0  0  0  0  0  0  0  0 16  0
AD  0  0  0  0  0  0  0  0  0 16  0  0  0  0 16  0  0  0 16  0  0  0
AE  0  0  0  0  0  0  0  0  0  0 16  0  0 16  0  0  0  0  0  0  0  0
AF  0  0  0  0  0  0  0  0  0  0  0 16  0  0  0  0 16  0  0  0  0  0
BC  0  0  0  0  0  0  0  0  0  0  0  0 16  0  0  0  0  0  0  0  0 16
BD  0  0  0  0  0  0  0  0  0  0 16  0  0 16  0  0  0  0  0  0  0  0
BE  0  0  0  0  0  0  0  0  0 16  0  0  0  0 16  0  0  0 16  0  0  0
BF  0  0  0  0  0  0  0  0  0  0  0  0  0  0  0 16  0 16  0  0  0  0
CD  0  0  0  0  0  0  0  0  0  0  0 16  0  0  0  0 16  0  0  0  0  0
CE  0  0  0  0  0  0  0  0  0  0  0  0  0  0  0 16  0 16  0  0  0  0
CF  0  0  0  0  0  0  0  0  0 16  0  0  0  0 16  0  0  0 16  0  0  0
DE  0  0  0  0  0  0  0 16  0  0  0  0  0  0  0  0  0  0  0 16  0  0
DF  0  0  0  0  0  0  0  0 16  0  0  0  0  0  0  0  0  0  0  0 16  0
EF  0  0  0  0  0  0  0  0  0  0  0  0 16  0  0  0  0  0  0  0  0 16

\end{verbatim}

\begin{verbatim}

       A  B  C  D  E  F AB AC AD AE AF BC BD BE BF CD CE CF DE DF EF
   16  0  0  0  0  0  0  0  0  0  0  0  0  0  0  0  0  0  0  0  0  0
A   0 16  0  0  0  0  0  0  0  0  0  0 16  0  0  0  0  0  0  0  0  0
B   0  0 16  0  0  0  0  0 16  0  0  0  0  0  0  0  0  0  0  0  0  0
C   0  0  0 16  0  0  0 16  0  0  0  0  0  0  0  0  0  0  0  0  0  0
D   0  0  0  0 16  0  0  0  0  0  0  0  0  0  0  0  0  0  0  0  0  0
E   0  0  0  0  0 16  0  0  0  0  0  0  0  0  0  0  0  0  0  0  0  0
F   0  0  0  0  0  0 16  0  0  0  0  0  0  0  0  0  0  0  0  0  0  0
AB  0  0  0 16  0  0  0 16  0  0  0  0  0  0  0  0  0  0  0  0  0  0
AC  0  0 16  0  0  0  0  0 16  0  0  0  0  0  0  0  0  0  0  0  0  0
AD  0  0  0  0  0  0  0  0  0 16  0  0  0  0  0  0  0  0  0  0  0 16
AE  0  0  0  0  0  0  0  0  0  0 16  0  0  0  0  0  0  0  0  0 16  0
AF  0  0  0  0  0  0  0  0  0  0  0 16  0  0  0  0  0  0  0 16  0  0
BC  0 16  0  0  0  0  0  0  0  0  0  0 16  0  0  0  0  0  0  0  0  0
BD  0  0  0  0  0  0  0  0  0  0  0  0  0 16  0  0  0  0  0  0  0  0
BE  0  0  0  0  0  0  0  0  0  0  0  0  0  0 16  0  0  0  0  0  0  0
BF  0  0  0  0  0  0  0  0  0  0  0  0  0  0  0 16  0  0  0  0  0  0
CD  0  0  0  0  0  0  0  0  0  0  0  0  0  0  0  0 16  0  0  0  0  0
CE  0  0  0  0  0  0  0  0  0  0  0  0  0  0  0  0  0 16  0  0  0  0
CF  0  0  0  0  0  0  0  0  0  0  0  0  0  0  0  0  0  0 16  0  0  0
DE  0  0  0  0  0  0  0  0  0  0  0 16  0  0  0  0  0  0  0 16  0  0
DF  0  0  0  0  0  0  0  0  0  0 16  0  0  0  0  0  0  0  0  0 16  0
EF  0  0  0  0  0  0  0  0  0 16  0  0  0  0  0  0  0  0  0  0  0 16
\end{verbatim}

\pagebreak

\begin{verbatim}

       A  B  C  D  E  F AB AC AD AE AF BC BD BE BF CD CE CF DE DF EF
   16  0  0  0  0  0  0  0  0  0  0  0  0  0  0  0  0  0  0  0  0  0
A   0 16  0  0  0  0  0  0  0  0  0  0  0  0  0  0  0  0  0  8  0 -8
B   0  0 16  0  0  0  0  0  0  0  0  0  0  0  0  0  0  0  0  0  0  0
C   0  0  0 16  0  0  0  0  0  0  0  0  0  0  0  0  0  0  0  8  0  8
D   0  0  0  0 16  0  0  0  0  0  8  0  0  0  0  0  0  8  0  0  0  0
E   0  0  0  0  0 16  0  0  0  8  0 -8  0  0  0  0  8  0  8  0  0  0
F   0  0  0  0  0  0 16  0  0  0 -8  0  0  0  0  0  0  8  0  0  0  0
AB  0  0  0  0  0  0  0 16  0  0  0  0  0  0  0  0  0  0  0 -8  0 -8
AC  0  0  0  0  0  0  0  0 16  0  0  0  0  0  0  0  0  0  0  0  0  0
AD  0  0  0  0  0  8  0  0  0 16  0  0  0  0 -8  0  0  0  0  0  0  0
AE  0  0  0  0  8  0 -8  0  0  0 16  0  0 -8  0 -8  0  0  0  0  0  0
AF  0  0  0  0  0 -8  0  0  0  0  0 16  0  0 -8  0  0  0  0  0  0  0
BC  0  0  0  0  0  0  0  0  0  0  0  0 16  0  0  0  0  0  0  8  0 -8
BD  0  0  0  0  0  0  0  0  0  0 -8  0  0 16  0  0  0  8  0  0  0  0
BE  0  0  0  0  0  0  0  0  0 -8  0 -8  0  0 16  0  8  0 -8  0  0  0
BF  0  0  0  0  0  0  0  0  0  0 -8  0  0  0  0 16  0 -8  0  0  0  0
CD  0  0  0  0  0  8  0  0  0  0  0  0  0  0  8  0 16  0  0  0  0  0
CE  0  0  0  0  8  0  8  0  0  0  0  0  0  8  0 -8  0 16  0  0  0  0
CF  0  0  0  0  0  8  0  0  0  0  0  0  0  0 -8  0  0  0 16  0  0  0
DE  0  8  0  8  0  0  0 -8  0  0  0  0  8  0  0  0  0  0  0 16  0  0
DF  0  0  0  0  0  0  0  0  0  0  0  0  0  0  0  0  0  0  0  0 16  0
EF  0 -8  0  8  0  0  0 -8  0  0  0  0 -8  0  0  0  0  0  0  0  0 16
\end{verbatim}
\end{small}

\subsubsection*{Case 5: \(N=24\)
  and \(m=7\)}
\begin{scriptsize}

 $(\pi_1, \pi_2)=(0.7, 0.3)$ and 
$b_3, b_4=(0, 35/9)$

\begin{verbatim}

        A  B  C  D  E  F  G A:B A:C A:D A:E A:F A:G B:C B:D B:E B:F B:G C:D C:E C:F C:G D:E D:F D:G E:F E:G F:G
    24  0  0  0  0  0  0  0   0   0   0   0   0   0   0   0   0   0   0   0   0   0   0   0   0   0   0   0   0
A    0 24  0  0  0  0  0  0   0   0   0   0   0   0   0   0   0   0   0   0   0   0   0   0   0   0   0   0   0
B    0  0 24  0  0  0  0  0   0   0   0   0   0   0   0   0   0   0   0   0   0   0   0   0   0   0   0   0   0
C    0  0  0 24  0  0  0  0   0   0   0   0   0   0   0   0   0   0   0   0   0   0   0   0   0   0   0   0   0
D    0  0  0  0 24  0  0  0   0   0   0   0   0   0   0   0   0   0   0   0   0   0   0   0   0   0   0   0   0
E    0  0  0  0  0 24  0  0   0   0   0   0   0   0   0   0   0   0   0   0   0   0   0   0   0   0   0   0   0
F    0  0  0  0  0  0 24  0   0   0   0   0   0   0   0   0   0   0   0   0   0   0   0   0   0   0   0   0   0
G    0  0  0  0  0  0  0 24   0   0   0   0   0   0   0   0   0   0   0   0   0   0   0   0   0   0   0   0   0
A:B  0  0  0  0  0  0  0  0  24   0   0   0   0   0   0   0   0   0   0  -8  -8  -8  -8  -8   8  -8  -8  -8   8
A:C  0  0  0  0  0  0  0  0   0  24   0   0   0   0   0  -8  -8  -8  -8   0   0   0   0   8  -8   8  -8   8   8
A:D  0  0  0  0  0  0  0  0   0   0  24   0   0   0  -8   0  -8   8  -8   0   8  -8   8   0   0   0   8   8   8
A:E  0  0  0  0  0  0  0  0   0   0   0  24   0   0  -8  -8   0  -8  -8   8   0  -8   8   0   8   8   0   0  -8
A:F  0  0  0  0  0  0  0  0   0   0   0   0  24   0  -8   8  -8   0   8  -8  -8   0   8   8   0   8   0  -8   0
A:G  0  0  0  0  0  0  0  0   0   0   0   0   0  24  -8  -8  -8   8   0   8   8   8   0   8   8   0  -8   0   0
B:C  0  0  0  0  0  0  0  0   0   0  -8  -8  -8  -8  24   0   0   0   0   0   0   0   0  -8  -8  -8   8  -8   8
B:D  0  0  0  0  0  0  0  0   0  -8   0  -8   8  -8   0  24   0   0   0   0  -8  -8  -8   0   0   0   8  -8  -8
B:E  0  0  0  0  0  0  0  0   0  -8  -8   0  -8  -8   0   0  24   0   0  -8   0   8  -8   0   8  -8   0   0  -8
B:F  0  0  0  0  0  0  0  0   0  -8   8  -8   0   8   0   0   0  24   0  -8   8   0   8   8   0  -8   0  -8   0
B:G  0  0  0  0  0  0  0  0   0  -8  -8  -8   8   0   0   0   0   0  24  -8  -8   8   0  -8  -8   0  -8   0   0
C:D  0  0  0  0  0  0  0  0  -8   0   0   8  -8   8   0   0  -8  -8  -8  24   0   0   0   0   0   0   8   8  -8
C:E  0  0  0  0  0  0  0  0  -8   0   8   0  -8   8   0  -8   0   8  -8   0  24   0   0   0   8   8   0   0   8
C:F  0  0  0  0  0  0  0  0  -8   0  -8  -8   0   8   0  -8   8   0   8   0   0  24   0   8   0  -8   0   8   0
C:G  0  0  0  0  0  0  0  0  -8   0   8   8   8   0   0  -8  -8   8   0   0   0   0  24   8  -8   0   8   0   0
D:E  0  0  0  0  0  0  0  0  -8   8   0   0   8   8  -8   0   0   8  -8   0   0   8   8  24   0   0   0   0  -8
D:F  0  0  0  0  0  0  0  0   8  -8   0   8   0   8  -8   0   8   0  -8   0   8   0  -8   0  24   0   0  -8   0
D:G  0  0  0  0  0  0  0  0  -8   8   0   8   8   0  -8   0  -8  -8   0   0   8  -8   0   0   0  24  -8   0   0
E:F  0  0  0  0  0  0  0  0  -8  -8   8   0   0  -8   8   8   0   0  -8   8   0   0   8   0   0  -8  24   0   0
E:G  0  0  0  0  0  0  0  0  -8   8   8   0  -8   0  -8  -8   0  -8   0   8   0   8   0   0  -8   0   0  24   0
F:G  0  0  0  0  0  0  0  0   8   8   8  -8   0   0   8  -8  -8   0   0  -8   8   0   0  -8   0   0   0   0  24
\end{verbatim}

\pagebreak

 $(\pi_1, \pi_2)=c(0.8, 0.8)$, 
  $b_3, b_4=c(2/3, 5/3)$
  
\begin{verbatim}
        A  B  C  D  E  F  G A:B A:C A:D A:E A:F A:G B:C B:D B:E B:F B:G C:D C:E C:F C:G D:E D:F D:G E:F E:G F:G
    24  0  0  0  0  0  0  0   0   0   0   0   0   0   0   0   0   0   0   0   0   0   0   0   0   0   0   0   0
A    0 24  0  0  0  0  0  0   0   0   0   0   0   0   0   8   0  -8   0   0   0   0   0   0   0   0   0   0   0
B    0  0 24  0  0  0  0  0   0   0   8   0  -8   0   0   0   0   0   0   0  -8   0  -8   0   8   0   0  -8   0
C    0  0  0 24  0  0  0  0   0   0   0   0   0   0   0   0  -8   0  -8   0   0   0   0   0   0   0   0   0   0
D    0  0  0  0 24  0  0  0   8   0   0   0   0   0   0   0   0   8   0   0   0   0   0   0   0   0   0   0   0
E    0  0  0  0  0 24  0  0   0   0   0   0   0   0  -8   0   0   0  -8   0   0   0   0   0   0   0   0   0   0
F    0  0  0  0  0  0 24  0  -8   0   0   0   0   0   0   8   0   0   0   0   0   0   0   0   0   0   0   0   0
G    0  0  0  0  0  0  0 24   0   0   0   0   0   0  -8   0  -8   0   0   0   0   0   0   0   0   0   0   0   0
A:B  0  0  0  0  8  0 -8  0  24   0   0   0   0   0   0   0   0   0   0   0   0   0   0   0   0   0   0   0   0
A:C  0  0  0  0  0  0  0  0   0  24   0   0   0   0   0   0   0   0   0   0   0   0   0  -8  -8   8  -8  -8   8
A:D  0  0  8  0  0  0  0  0   0   0  24   0   0   0   0   0   0   0   0   0  -8  -8   8   0   0   0  -8   8  -8
A:E  0  0  0  0  0  0  0  0   0   0   0  24   0   0   0   0   0   0   0  -8   0  -8  -8   0  -8   8   0   0  -8
A:F  0  0 -8  0  0  0  0  0   0   0   0   0  24   0   0   0   0   0   0  -8  -8   0   8  -8   0  -8   0  -8   0
A:G  0  0  0  0  0  0  0  0   0   0   0   0   0  24   0   0   0   0   0   8  -8   8   0   8  -8   0  -8   0   0
B:C  0  0  0  0  0 -8  0 -8   0   0   0   0   0   0  24   0   0   0   0   0   0   0   0   0   0   0   0   0   0
B:D  0  8  0  0  0  0  8  0   0   0   0   0   0   0   0  24   0   0   0   0   0   0   0   0   0   0   0   0   0
B:E  0  0  0 -8  0  0  0 -8   0   0   0   0   0   0   0   0  24   0   0   0   0   0   0   0   0   0   0   0   0
B:F  0 -8  0  0  8  0  0  0   0   0   0   0   0   0   0   0   0  24   0   0   0   0   0   0   0   0   0   0   0
B:G  0  0  0 -8  0 -8  0  0   0   0   0   0   0   0   0   0   0   0  24   0   0   0   0   0   0   0   0   0   0
C:D  0  0  0  0  0  0  0  0   0   0   0  -8  -8   8   0   0   0   0   0  24   0   0   0   0   0   0   8   8   8
C:E  0  0 -8  0  0  0  0  0   0   0  -8   0  -8  -8   0   0   0   0   0   0  24   0   0   0   8   8   0   0  -8
C:F  0  0  0  0  0  0  0  0   0   0  -8  -8   0   8   0   0   0   0   0   0   0  24   0   8   0   8   0  -8   0
C:G  0  0 -8  0  0  0  0  0   0   0   8  -8   8   0   0   0   0   0   0   0   0   0  24   8   8   0  -8   0   0
D:E  0  0  0  0  0  0  0  0   0  -8   0   0  -8   8   0   0   0   0   0   0   0   8   8  24   0   0   0   0  -8
D:F  0  0  8  0  0  0  0  0   0  -8   0  -8   0  -8   0   0   0   0   0   0   8   0   8   0  24   0   0  -8   0
D:G  0  0  0  0  0  0  0  0   0   8   0   8  -8   0   0   0   0   0   0   0   8   8   0   0   0  24  -8   0   0
E:F  0  0  0  0  0  0  0  0   0  -8  -8   0   0  -8   0   0   0   0   0   8   0   0  -8   0   0  -8  24   0   0
E:G  0  0 -8  0  0  0  0  0   0  -8   8   0  -8   0   0   0   0   0   0   8   0  -8   0   0  -8   0   0  24   0
F:G  0  0  0  0  0  0  0  0   0   8  -8  -8   0   0   0   0   0   0   0   8  -8   0   0  -8   0   0   0   0  24


\end{verbatim}

\end{scriptsize}

\end{document}
